# Supplementary material for: Direct numerical simulation of thermo-diffusively unstable premixed hydrogen-air flames in a fully-developed turbulent channel flow at $Re_\tau=530$
Source: arXiv:2511.20930 ancillary file (2025-11-27)
Supplement: Supplementary file 1 [file Supplementary_Material.pdf]

# Supplementary to manuscript: Direct numerical simulation of thermo-diffusively unstable premixed hydrogen-air flames in a fully-developed turbulent channel flow at $Re_\tau = 530$

Felix Rong[a,*], Max Schneider[a],
Hendrik Nicolai[a], Christian Hasse[a], Andrea Gruber[b, c]

[a]*Technical University of Darmstadt, Department of Mechanical Engineering, Simulation of Reactive Thermo-Fluid Systems, Otto-Berndt-Str. 2, 64287 Darmstadt, Germany*
[b]*SINTEF Energy Research, Thermal Energy Department, 7465 Trondheim, Norway.*
[c]*Norwegian University of Science and Technology, Department of Energy and Process Engineering, 7491 Trondheim, Norway.*

[*]*Corresponding author: rong@stfs.tu-darmstadt.de*

---

This supplementary document contains:

- **S1**: Simulations of laminar, thermo-diffusively unstable flames under the conditions of the present study
  - **S1.1**: Linear regime and dispersion relation
  - **S1.2**: Non-linear regime and stretch factor $I_0$

## S1. Laminar thermo-diffusively unstable flames

Two-dimensional (2D) laminar freely propagating (FP) flames are simulated to evaluate the characteristic properties of thermo-diffusive (TD) instabilities and to quantify the laminar reference value of the stretch factor $I_0$ under the conditions of the present study.

### *S1.1. Dispersion relation (linear stability analysis)*

The evolution of TD-unstable flames can be differentiated into linear and non-linear regimes (Altantzis *et al.*, 2012; Berger *et al.*, 2023). The linear regime is analysed through a linear stability analysis, where the flame amplitude exhibits exponential growth over time with the growth rate $\omega$. To numerically examine the development of the instability over time, a small sinusoidal perturbation with an amplitude $a_0 = 0.04\,\delta_\mathrm{F}$ is imposed on the planar flame front, as shown in the configuration in figure S1. Here, the domain size $L_y$ in the lateral direction is kept equal to the perturbation wavelength $\lambda_\mathrm{pert}$, so that exactly one wavelength of the prescribed perturbation fits exactly into the domain. Further details on the methodology can be found, for example, in the work of Berger *et al.* (2022); Lulic *et al.* (2023).

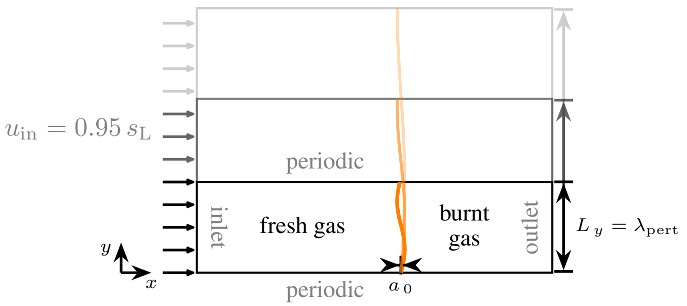


Figure S1: Schematic of the two-dimensional laminar freely propagating flame configuration. The varying domain size, $L_y = \lambda_\mathrm{pert}$, in the lateral direction is illustrated using different shades of grey, and the orange colour denotes the flame front.

The dispersion relation, which describes the growth rate of different wavelengths of a harmonic perturbation, is shown in figure S2 for the $\varphi = 0.25$ and $\varphi = 0.35$ flames. Additionally, the growth rate for pure hydrodynamic instability (also referred to as Darrieus-Landau instability, (Matalon, 2007)) is shown as dashed lines, confirming that both flames are TD-unstable. The characteristic scales of TD instabilities are listed in table S1 for both flames.

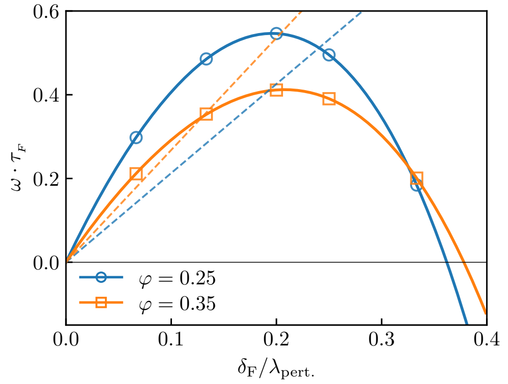


Figure S2: Dispersion relations of two-dimensional laminar flame with the dashed lines denoting the hydrodynamic Darrieus-Landau instability. The dispersion relation is shown in non-dimensionalized form using the flame thickness $\delta_\mathrm{F}$ and flame time $\tau_\mathrm{F}$, respectively.

| | $\varphi = 0.25$ | $\varphi = 0.35$ |
|---|---|---|
| $\lambda_\mathrm{crit}\,/\,\delta_\mathrm{F}$ | 2.768 | 2.644 |
| $\lambda_{\omega_\mathrm{max}}\,/\,\delta_\mathrm{F}$ | 5.076 | 4.812 |
| $(\omega\,\tau_F)_\mathrm{max}$ | 0.549 | 0.412 |

Table S1: Characteristic scales of TD flame instability: critical wavelength $\lambda_\mathrm{crit}$, most unstable wavelength $\lambda_{\omega_\mathrm{max}}$ and maximal growth rate $\omega_\mathrm{max}$ corresponding to figure S2. The values are non-dimensionalized by the flame thickness $\delta_\mathrm{F}$ and flame time $\tau_\mathrm{F}$, respectively.

*S1.2. Non-linear regime and stretch factor $I_0$*

In the non-linear regime, the laminar flame front exhibits pronounced flame wrinkling and cell formation, with a non-linear temporal evolution of flame surface and flame speed. Figure S3 shows the instantaneous flame structure of the 2D unstable FP flames in a sufficiently large computational domain. For both equivalence ratios, the normalized temperature, mixture fraction and mass fraction of OH radical are shown. The effects of TD instabilities are more pronounced for the leaner $\varphi = 0.25$ flame, as larger magnitudes of normalised temperature, mixture variation, and local reactivity (presented by the OH radical mass fraction) are observed. Furthermore, distinct cusps, typical for TD instabilities, are clearly present in the laminar $\varphi = 0.25$ flame. For both flames, significant local increases in mixture fraction and OH mass fraction occur, while the maximum temperatures only slightly exceed the respective adiabatic flame temperature ($T_{\mathrm{norm}} > 1$), accompanied by a low value of the stretch factor $I_0$, that is minimally above unity. Based on these observations and the dispersion relations in figure S2, it can be concluded that the $\varphi = 0.35$ laminar FP flame is moderately TD-unstable, while the $\varphi = 0.35$ laminar FP flame is weakly TD-unstable. These findings are in agreement with studies in the literature, showing that TD instabilities are damped and the value of the stretch factor is significantly reduced with preheated unburnt gas temperature (Berger *et al.*, 2022; Rieth *et al.*, 2023).

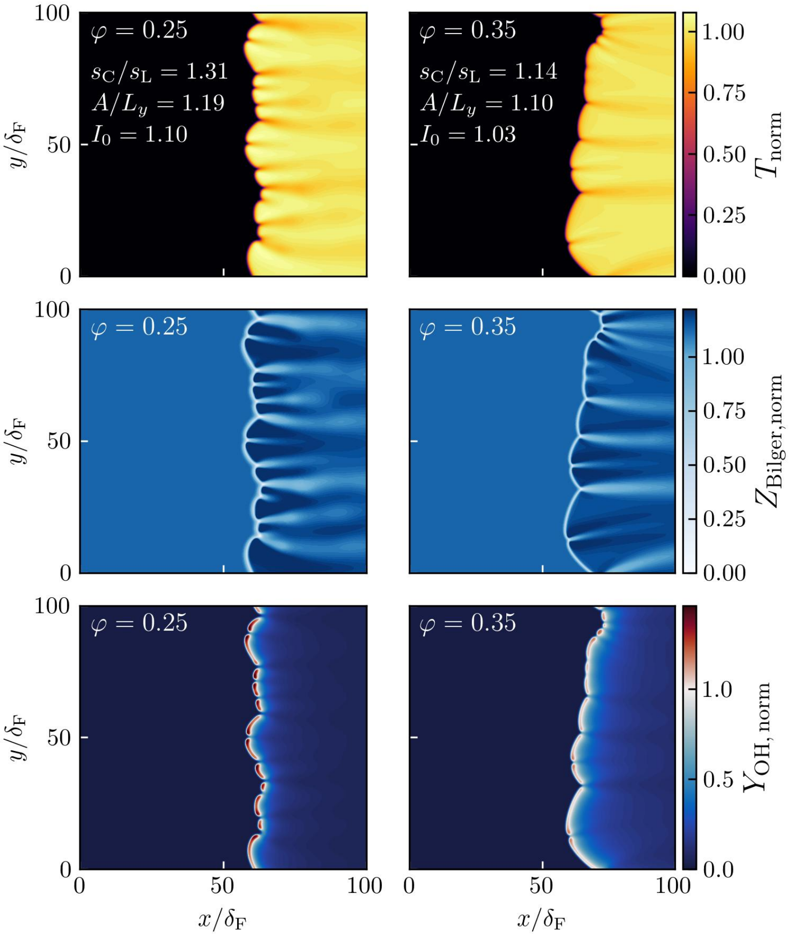


Figure S3: Flame structure of instantaneous 2D FP flames for both equivalence ratios $\varphi = 0.25$ (left) and $\varphi = 0.35$ (right). The average flame speed enhancement (consumption speed $s_c$ over laminar burning velocity $s_L$), the flame surface area increase (flame front length $A$ over the longitudinal domain size $L_y$) and the stretch factor $I_0$ are annotated.

The stretch factor $I_0$ quantifies the flame speed enhancement that is not resulting from the increase in flame surface area and can be interpreted as a marker for TD instabilities. As shown in the work of Berger *et al.* (2019),

the value of the stretch factor $I_0$ depends strongly on the lateral domain size $L_y$, since it acts as a geometric restriction for the wavelengths of possible perturbations. In figure S4, the resulting values of $I_0$ are shown for different domain sizes for both flames. The domain size corresponding to the maximum value of $I_0$ is close to the most unstable wavelength.

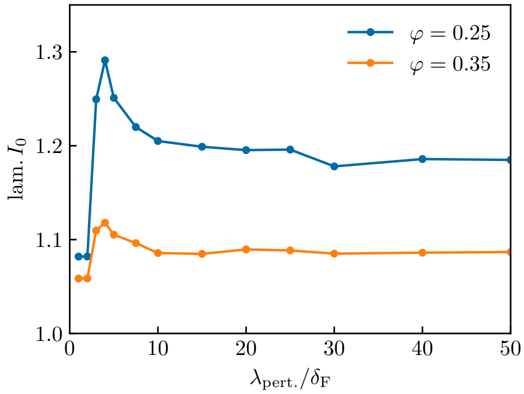


Figure S4: Stretch factor $I_0$ of 2D laminar FP flames as a function of the lateral domain size $L_y = \lambda_{\mathrm{pert}}$.

## References


Altantzis, C., Frouzakis, C. E., Tomboulides, A. G., Matalon, M. & Boulouchos, K. 2012 Hydrodynamic and thermodiffusive instability effects on the evolution of laminar planar lean premixed hydrogen flames. *J. Fluid Mech.* **700**, 329–361.

Berger, L., Attili, A. & Pitsch, H. 2022 Intrinsic instabilities in premixed hydrogen flames: Parametric variation of pressure, equivalence ratio, and temperature. part 1 - dispersion relations in the linear regime. *Combust. Flame* **240**, 111935.

Berger, L., Grinberg, M., Jürgens, B., Lapenna, P. E., Creta, F., Attili, A. & Pitsch, H. 2023 Flame fingers and interactions of hydrodynamic and thermodiffusive instabilities in laminar lean hydrogen flames. *P. Combust. Inst.* **39** (2), 1525–1534.

Berger, L., Kleinheinz, K., Attili, A. & Pitsch, H. 2019 Characteristic patterns of thermodiffusively unstable premixed lean hydrogen flames. *P. Combust. Inst.* **37** (2), 1879–1886.

Lulic, H., Breicher, A., Scholtissek, A., Lapenna, P. E., Dreizler, A., Creta, F., Hasse, C., Geyer, D. & Ferraro, F. 2023 On polyhedral structures of lean methane/hydrogen bunsen flames: Combined experimental and numerical analysis. *P. Combust. Inst.* **39** (2), 1977–1986.

Matalon, M. 2007 Intrinsic Flame Instabilities in Premixed and Nonpremixed Combustion. *Annu. Rev. Fluid Mech.* **39** (1), 163–191.

Rieth, M., Gruber, A. & Chen, J. H. 2023 The effect of pressure on lean premixed hydrogen-air flames. *Combust. Flame* **250**, 112514.
